# Supplementary material for: Sketch2code: Generating a website from a paper mockup
Source: arXiv:1905.13750 source file (2019-05-09)
Supplement: Supplementary file 1 [file appendix.tex]

% \section{TODO}
% Some text for the appendix.
